# Supplementary material for: Democracy and Growth in the 21st Century
Source: arXiv:2104.07617 source file (2025-04-24)
Supplement: Supplementary file 1 [file 19_causal_mediation_analysis.tex]

\begin{table}\centering 
  \caption{ Causal Mediation Analysis of Potential Policy Mechanisms in 2020}
  \label{tab:causal-mediation} 
  \begin{threeparttable}
\begin{tabularx}{\textwidth}{{l}*{1}{Y} {c}*{3}{Y}}
\hline\hline
 & (1) & (2) & (3) \\
                % &\multicolumn{1}{c}{(1)}         &\multicolumn{1}{c}{(2)}         &\multicolumn{1}{c}{(3)}         \\
                &     Severity         &     Coverage        &    Speed       \\
\hline  \\[-1.8ex]
% \multicolumn{4}{c}{\textbf{Panel A: GDP Growth Rates in 2020}} \\  \\
\textbf{Panel A} & \multicolumn{3}{c}{Dependent Variable is GDP Per Capita Growth Rate in 2020} \\ \cline{2-4}  \\[-1.8ex]
Total Effect of Democracy  &     -2.7 &     -2.7        &     -2.7        \\
                &      (2.1)            &   (2.1)        &    (2.1)       \\
Direct Effect of Democracy    &     -1.4    &     -1.4         &     -1.5         \\
                &     (1.0)     &    (0.8)         &    (0.8)         \\
Indirect Effect Through Mediator &   -1.3      &     -1.2        &     -1.1        \\
                &      (2.8)             &    (2.6)         &   (2.6)         \\

\hline \\[-1.8ex]

\textbf{Panel B} & \multicolumn{3}{c}{Dependent Variable is Covid-19 Deaths Per Million in 2020} \\ \cline{2-4}  \\[-1.8ex]
        
Total Effect of Democracy         &    468.0  &     468.0   &     468.0   \\
             &  (126.5)         &  (126.5)            & (126.5)  \\
Direct Effect of Democracy    &    120.6 &    143.0  &      165.3        \\
                &  (80.1)        &   (69.5)           &   (115.6)        \\
Indirect Effect Through Mediator     &     347.4        &     325.0       &    302.7          \\
                 & (190.5)         &  (173.9)       &  (329.2)         \\
                 
 \hline \\[-1.8ex] 
N     &       80         &       80         &       80         \\

\hline\hline
\end{tabularx}
\begin{tablenotes} 
\item {\footnotesize {\textit{Notes:} This table reports the results of causal mediation analyses of democracy's effect on each outcome in 2020 with three potential mediators: severity, coverage, and speed of policy responses. All regressions use log European settler mortality as an IV. 
\input{supporting_files/coefs/explanation_dem} We proxy for severity by Oxford COVID-19 Government Response Tracker's Containment Health Index at the 10th confirmed Covid-19 case, for coverage by the number of domains the policy covers at the 10th confirmed Covid-19 case, and for speed by the number of days between the 10th case of Covid-19 and the date when the government introduces any containment measure. This analysis implements the causal mediation analysis framework for linear IV models introduced by Dippel et al. (2020). It estimates three effects: (i) the total effect of a single treatment variable (democracy) on the outcome (GDP per capita growth rates in 2020 or Covid-19 deaths per million in 2020), where the treatment variable is instrumented by a single IV (log European settler mortality), (ii) the direct effect of treatment on the outcome, net of the effect of the mediator, and (iii) the indirect effect (mediation effect) of a mediator (severity, coverage or speed of initial response) through which the treatment variable affects the outcomes. %The key assumption is that treatment is endogenous in a regression of outcomes on treatment primarily because of omitted variables that affect the mediator. 
Under linearity, the resulting identification framework is estimated using three separate 2SLS estimations of the effect of treatment on the mediator, the effect of treatment on the outcome, and the effect of the mediator on the outcome conditional on treatment. All regressions are unweighted. The estimates in this table are slightly different from those in Table \ref{tab:2sls-compare-weighting} because this table uses only observations for which data for all mediators are available. Robust standard errors are in parentheses.
\input{supporting_files/coefs/explanation_n}}
\end{tablenotes}
\end{threeparttable}
\end{table}
