# Supplementary material for: Democracy and Growth in the 21st Century
Source: arXiv:2104.07617 source file (2025-04-24)
Supplement: Supplementary file 2 [file 12_2sls_exclude_US_China_mean_death_per_million_20_22_panelA1.tex]

Democracy Index (V-Dem, 2019)&       355.0&       417.7&       357.6&       374.3&       294.6&       322.1&       420.3&       405.2&       277.1&       339.5&       341.5&       378.3\\
&      (63.0)&      (91.8)&      (62.6)&      (24.8)&      (74.7)&      (45.2)&     (120.5)&      (65.8)&      (60.4)&      (38.3)&      (48.9)&      (25.3)\\
Include US \& China? & \cmark & \cmark  & \cmark & \cmark & \cmark & \cmark  & \cmark & \cmark & \cmark & \cmark & \cmark & \cmark\\
N                   &          81&          81&          86&          86&          90&          90&         132&         132&         138&         138&          71&          71\\
