# Supplementary material for: Democracy and Growth in the 21st Century
Source: arXiv:2104.07617 source file (2025-04-24)
Supplement: Supplementary file 3 [file 12_2sls_exclude_US_China_mean_death_per_million_20_22_panelA2.tex]

Democracy Index (V-Dem, 2019)&       388.7&       842.8&       257.1&       362.0&     -6664.4&     -7338.8&       413.3&       480.3&       172.6&        36.2&       281.8&       416.2\\
&     (142.2)&     (576.2)&     (158.5)&     (276.5)&   (35530.9)&   (28569.0)&     (189.5)&     (207.5)&     (110.7)&     (168.2)&     (127.0)&     (133.3)\\
Include US \& China? & \xmark & \xmark  & \xmark & \xmark   & \xmark & \xmark  & \xmark & \xmark  & \xmark & \xmark  & \xmark & \xmark \\
N                   &          79&          79&          84&          84&          88&          88&         130&         130&         136&         136&          69&          69\\
\hline \\[-1.8ex] IVs & \multicolumn{2}{c}{settler mortality} &  \multicolumn{2}{c}{population density} & \multicolumn{2}{c}{legal origin} & \multicolumn{2}{c}{language} & \multicolumn{2}{c}{crops \& minerals}  & \multicolumn{2}{c}{all IVs}  \\ Baseline Controls & \xmark & \cmark & \xmark & \cmark & \xmark & \cmark & \xmark & \cmark & \xmark & \cmark & \xmark & \cmark\\
