# Supplementary material for: Democracy and Growth in the 21st Century
Source: arXiv:2104.07617 source file (2025-04-24)
Supplement: Supplementary file 4 [file rf_mean_growth_rate_1981_2000.tex]

\begin{tabular}{l*{12}{c}}
\hline\hline
                    &\multicolumn{1}{c}{(1)}&\multicolumn{1}{c}{(2)}&\multicolumn{1}{c}{(3)}&\multicolumn{1}{c}{(4)}&\multicolumn{1}{c}{(5)}&\multicolumn{1}{c}{(6)}&\multicolumn{1}{c}{(7)}&\multicolumn{1}{c}{(8)}&\multicolumn{1}{c}{(9)}&\multicolumn{1}{c}{(10)}&\multicolumn{1}{c}{(11)}&\multicolumn{1}{c}{(12)}\\
\hline
Log European Settler Mortality&         0.5&         0.7&            &            &            &            &            &            &            &            &        -0.6&        -0.3\\
                    &       (0.3)&       (0.6)&            &            &            &            &            &            &            &            &       (0.8)&       (0.5)\\
Log Population Density in 1500s&            &            &         0.4&         1.0&            &            &            &            &            &            &         0.5&         0.9\\
                    &            &            &       (0.2)&       (0.3)&            &            &            &            &            &            &       (0.3)&       (0.2)\\
British Legal Origin&            &            &            &            &        -0.6&        -0.5&            &            &            &            &        -2.2&        -0.8\\
                    &            &            &            &            &       (1.2)&       (1.2)&            &            &            &            &       (1.6)&       (0.6)\\
Fraction Speaking English&            &            &            &            &            &            &         1.1&         0.5&            &            &         3.3&         0.5\\
                    &            &            &            &            &            &            &       (0.2)&       (0.5)&            &            &       (2.2)&       (1.5)\\
Fraction Speaking European&            &            &            &            &            &            &        -1.2&        -0.6&            &            &        -2.7&        -1.0\\
                    &            &            &            &            &            &            &       (0.6)&       (0.4)&            &            &       (2.4)&       (0.8)\\
Bananas             &            &            &            &            &            &            &            &            &         1.2&         1.1&       -0.03&         0.7\\
                    &            &            &            &            &            &            &            &            &       (0.6)&       (0.6)&       (0.7)&       (0.7)\\
Coffee              &            &            &            &            &            &            &            &            &         0.2&        0.05&         0.2&        -1.4\\
                    &            &            &            &            &            &            &            &            &       (0.2)&       (0.5)&       (0.6)&       (1.0)\\
Copper              &            &            &            &            &            &            &            &            &         0.3&        -0.3&         0.3&         0.7\\
                    &            &            &            &            &            &            &            &            &       (0.4)&       (0.4)&       (1.3)&       (0.8)\\
Maize               &            &            &            &            &            &            &            &            &        -0.6&        -0.8&        -1.4&        -1.5\\
                    &            &            &            &            &            &            &            &            &       (0.4)&       (0.6)&       (3.1)&       (0.9)\\
Millet              &            &            &            &            &            &            &            &            &         0.9&         0.5&         0.9&        -1.2\\
                    &            &            &            &            &            &            &            &            &       (0.6)&       (0.4)&       (1.1)&       (1.0)\\
Rice                &            &            &            &            &            &            &            &            &        -1.0&         0.1&        -1.4&         1.0\\
                    &            &            &            &            &            &            &            &            &       (0.5)&       (0.7)&       (2.1)&       (1.0)\\
Rubber              &            &            &            &            &            &            &            &            &         1.8&         2.1&         0.6&         1.6\\
                    &            &            &            &            &            &            &            &            &       (1.5)&       (1.3)&       (0.8)&       (0.9)\\
Silver              &            &            &            &            &            &            &            &            &     -0.0003&        -0.2&         0.6&        -0.2\\
                    &            &            &            &            &            &            &            &            &       (0.3)&       (0.5)&       (1.1)&       (0.8)\\
Sugarcane           &            &            &            &            &            &            &            &            &        -0.5&        0.06&       -0.01&         1.2\\
                    &            &            &            &            &            &            &            &            &       (0.9)&       (0.8)&       (2.0)&       (1.1)\\
Wheat               &            &            &            &            &            &            &            &            &        -0.2&        -1.1&        -0.4&        -1.1\\
                    &            &            &            &            &            &            &            &            &       (1.1)&       (0.9)&       (1.3)&       (0.9)\\
 \hline \\[-1.8ex]Baseline Controls & \xmark & \cmark & \xmark & \cmark & \xmark & \cmark & \xmark & \cmark & \xmark & \cmark  & \xmark & \cmark  \\
N                   &          76&          76&          80&          80&          83&          83&         119&         119&         124&         124&          68&          68\\
\hline\hline
\end{tabular}
